# Supplementary material for: The intrinsic bispectrum of the Cosmic Microwave Background [PhD thesis]
Source: arXiv:1405.2280 source file (2015-12-03)
Supplement: Supplementary file 1 [file appendix_equations.tex]

%!TEX root = phd_thesis.tex

\chapter{The Boltzmann and Einstein equations}
\label{ch:appendix_equations}

Equationsssss.

The quadratic sources in real space, on the contrary, are unambiguous. For the time-time equation they are given by
\begin{align}
  % ~~~~~~~~~~~~~~~~~~~~
  & % Time-time (quad)
  % ~~~~~~~~~~~~~~~~~~~~
  \begin{aligned}
  \I\QTT \;=\; 
  &-12\,\Hc^2\,\I\Psi^2
  \;-\;8\,\I\Phi\,\partial^i\,\partial_i\I\Phi \;-\; 3\,\partial_i\I\Phi\partial^i\I\Phi \nmsk
  &+12\,\Hc\,\I\Phid \, (\I\Phi - \I\Psi)
  \;-\;3\,(\I\Phid)^2
  \end{aligned}
  \displaybreak[0]
  % ~~~~~~~~~~~~~~~~~~~~
  \msk& % Trace (quad)
  % ~~~~~~~~~~~~~~~~~~~~
  \begin{aligned}
  \I\QTR \;=\;
  &-12\,\I\Psi^2\,(\Hc^2\,+\,2\,\dot\Hc)
  \;-\;4\,\I\Psi\,\partial^i\,\partial_i\I\Psi \;-\; 2\,\partial_i\I\Phi\partial^i\I\Phi \nmsk
  &\;-\;8\,\I\Phi\,\partial^i\,\partial_i\I\Phi \;-\; 3\,\partial_i\I\Phi\partial^i\I\Phi
  \;+\;4\,\I\Phi\,\partial^i\,\partial_i\I\Psi \;-\; 2\,\partial_i\I\Phi\partial^i\I\Psi \nmsk
  &\;+\;12\,\I\Phidd\,(\I\Phi - \I\Psi)
  \;+\;24\,\Hc\,\I\Phid\,(\I\Phi - \I\Psi) \nmsk
  &\;-\; 6\,\I\Psid\,(4\,\Hc\,\I\Psi\,+\,\I\Phid)
  \;+\;3\,(\I\Phid)^2
  \end{aligned}
  % ~~~~~~~~~~~~~~~~~~~~~~~
  \msk& % Space-time (quad)
  % ~~~~~~~~~~~~~~~~~~~~~~~
  \begin{aligned}
  \I\QST \;=\;
  &-12\,\I\Psi^2\,(\Hc^2\,+\,2\,\dot\Hc)
  \;-\;4\,\I\Psi\,\partial^i\,\partial_i\I\Psi \;-\; 2\,\partial_i\I\Phi\partial^i\I\Phi \nmsk
  &\;-\;8\,\I\Phi\,\partial^i\,\partial_i\I\Phi \;-\; 3\,\partial_i\I\Phi\partial^i\I\Phi
  \;+\;4\,\I\Phi\,\partial^i\,\partial_i\I\Psi \;-\; 2\,\partial_i\I\Phi\partial^i\I\Psi \nmsk
  &\;+\;12\,\I\Phidd\,(\I\Phi - \I\Psi)
  \;+\;24\,\Hc\,\I\Phid\,(\I\Phi - \I\Psi) \nmsk
  &\;-\; 6\,\I\Psid\,(4\,\Hc\,\I\Psi\,+\,\I\Phid)
  \;+\;3\,(\I\Phid)^2
  \end{aligned}
\end{align}
For the space-time sources, we show the quadratic part of $\partial_i\,G^i_{\,0}$ rather than ${\QST}_{[m]}=\xivector{m}{i}\,G_{i0}$.
